# Supplementary material for: Federated Learning via Decentralized Dataset Distillation in Resource-Constrained Edge Environments
Source: arXiv:2208.11311 source file (2023-05-19)
Supplement: Supplementary file 1 [file A_notations.tex]

\section{Abbreviations and Notations}
\label{subsec:A}

We provide overviews of the most relevant notations and abbreviations in Tab.~\ref{table:notation} and Tab.~\ref{table:abbreviation}, respectively.

\setcounter{table}{0}

\begin{table*}[ht!]
\centering
\begin{threeparttable}
\caption{\centering Summary of mainly used notations in this paper.}
\label{table:notation}
\begin{tabular}{M{1.5cm}L{10.9cm}M{2cm}}
   \toprule %%%%%%%%%%%%%%%%%%
    \centering\textbf{Notation} & \centering\textbf{Meaning}  & \textbf{Navigation}\\
    \midrule %%%%%%%%%%%%%%%%%%

    $m$  & Number of clients in federated learning systems, $m \in \mathbb{N}_+$ & Sec.~3 \\

    $k$  & Index of a set of clients,  $k \in \mathbb{N}_+, 1 \leq k \leq m $  & Sec.~3\\
    
    $\mathcal{D}$ & Global dataset, see Eq.~\ref{Eq:D} & Sec.~3\\
    
    $\mathcal{D}_k$ & Local dataset in the client $k$, see Eq.~\ref{Eq:D_k} & Sec.~3\\
     
    $\mathcal{\tilde D}$ & Aggregated distilled dataset in the server, see Eq.~\ref{Eq:D_d} & Sec.~3\\
    
    $\mathcal{\tilde D}_k$ &  Distilled dataset in local dataset in the client $k$, see Eq.~\ref{Eq:D_kd} & Sec.~3\\

    $n$  & Number of data points in global dataset, $n=|\mathcal{D}_k|$ & Sec.~3 \\
    
    $n_k$  & Number of data points in local dataset in the client $k$, $n=|\mathcal{D}|$ & Sec.~3 \\
    
    $\tilde n$  & Number of aggregated distilled data points in the server, $n=|\mathcal{\tilde D}|$ & Sec.~3 \\
    
    $\tilde n_k$  & Number of distilled data points from the client $k$, $n=|\mathcal{\tilde D}_k|$ & Sec.~3 \\

    $i$, $j$  & Index of data points & Sec.~3 \\
    
    $s$  & Index of class of labeled data points & Sec.~3 \\
    
    $S$  & A set of classes of a labeled dataset, $s\in S$ & Sec.~3 \\
    
    $S_k$  & A set of classes of a labeled local dataset in the client $k$, $S_k\subseteq S$ & Sec.~3 \\

    $C_k$  & Number of classes in client $k$, $C_k = |S_k|$ & Sec.~3 \\
    
    $X$  & Matrix of stacked data points $x$, see Eq.~\ref{Eq:X} & Sec.~3 \\
    
    $X_k$  &  Matrix of stacked data points $x_k$, see Eq.~\ref{Eq:X_k} & Sec.~3 \\
    
    $\tilde X$  &  Matrix of stacked data points $\tilde x$, see Eq.~\ref{Eq:X_d} & Sec.~3 \\
    
    $\tilde X_k$  &  Matrix of stacked data points $\tilde x_k$, see Eq.~\ref{Eq:X_kd} & Sec.~3 \\

    $y_i$ & The label of the data point $i$ & Sec.~3\\
    
    $y_k$ & The label vector in the client $k$  & Sec.~3\\

    $\Theta$ & Hyper-parameters in kernel function  & Sec.~3\\
    
    $\Theta_k$ & Hyper-parameters in kernel function  & Sec.~3\\

    $e$ & Index of epochs   & Sec.~3\\

    $E$ & Index of the global training epochs  & Sec.~3\\

    $e_k$ & Index of the local distilling (training) epochs & Sec.~3\\

    $E_k$ & Number of the local distilling (training) epochs & Sec.~3\\
    
    $b$ & Index of batches & Sec.~3\\
    
    $X_b$ & Matrix of stacked data points in the batch $b$ & Sec.~3\\
    
    $y_b$ &  Label vector of the batch $b$ & Sec.~3\\

    $\mathcal{\tilde B}_k$ &  Batch set of synthetic data points for the distilling in the client $k$  & Sec.~3\\
    
    $\mathcal{\tilde B}$ & Batch set of aggregated distilled data points for the training in the server & Sec.~3\\
    
    $t$ &  Index of the communication rounds  & Sec.~3\\
    
    $T$ & Number of the communication rounds  & Sec.~3\\
    
%    $K_k$ &  Kernel function of KIP-based instance in the local client $k$ & Sec.~3\\
    
    $\eta$ & Global learning rate  & Sec.~3\\
    
    $\eta_k$ & Local learning rate in the client $k$ & Sec.~3\\
    
    $V_t$ & Communication volume (bit) in the communication round $t$ & Sec.~3\\
    
    $P$ & Bit size of models & Sec.~4\\

    \bottomrule %%%%%%%%%%%%%%%%%%
\end{tabular}
\end{threeparttable}
\end{table*}
\newcommand{\vecline}{~~~\rule[.5ex]{2em}{0.4pt}~~~}

\begin{minipage}[t]{0.5\textwidth}
\begin{equation}
    \label{Eq:D}
    \mathcal{D} = \{x_i|i=1,2,...,n \}
\end{equation}
\end{minipage}
\begin{minipage}[t]{0.5\textwidth}
\begin{equation}
    \label{Eq:D_k}
    \mathcal{D}_k = \{x_{k,i}|i=1,2,...,n_k \}
\end{equation}
\end{minipage}

\begin{minipage}[t]{0.5\textwidth}
\begin{equation}
    \label{Eq:D_d}
    \mathcal{\tilde D} = \{\tilde x_{j}|j=1,2,...,\tilde n \}
\end{equation}

\end{minipage}
\begin{minipage}[t]{0.5\textwidth}
\begin{equation}
    \label{Eq:D_kd}
    \mathcal{\tilde D}_k = \{\tilde x_{k,j}|j=1,2,...,\tilde n_k \}
\end{equation}
\end{minipage}

\begin{minipage}[t]{0.5\textwidth}

\begin{equation}
    \label{Eq:X}
    X = 
  \begin{bmatrix}
  \vecline x_{1} \vecline \\
  \vdots \\
  \vecline x_{i} \vecline \\
  \vdots\\
  \vecline x_{n} \vecline \\
  \end{bmatrix}
\end{equation}

\end{minipage}
\begin{minipage}[t]{0.5\textwidth}

\begin{equation}
    \label{Eq:X_k}
    X_k = 
  \begin{bmatrix}
  \vecline x_{k,1} \vecline \\
  \vdots \\
  \vecline x_{k,i} \vecline \\
  \vdots\\
  \vecline x_{k,n} \vecline \\
  \end{bmatrix}
\end{equation}

\end{minipage}

\begin{minipage}[t]{0.5\textwidth}

\begin{equation}
    \label{Eq:X_d}
    \tilde X = 
  \begin{bmatrix}
  \vecline \tilde x_{1} \vecline \\
  \vdots \\
  \vecline \tilde x_{j} \vecline \\
  \vdots\\
  \vecline \tilde x_{n} \vecline \\
  \end{bmatrix}
\end{equation}

\end{minipage}
\begin{minipage}[t]{0.5\textwidth}

\begin{equation}
    \label{Eq:X_kd}
    \tilde X_k = 
  \begin{bmatrix}
  \vecline \tilde x_{k,1} \vecline \\
  \vdots \\
  \vecline \tilde x_{k,j} \vecline \\
  \vdots\\
  \vecline \tilde x_{k,n} \vecline \\
  \end{bmatrix}
\end{equation}

\end{minipage}

\begin{table*}[ht!]
\centering
\begin{threeparttable}
\caption{\centering Summary of mainly used abbreviations in this paper.}
\label{table:abbreviation}
\begin{tabular}{M{1.8cm}L{10.7cm}M{2cm}}
   \toprule %%%%%%%%%%%%%%%%%%
    \centering\textbf{Abbr.} & \centering\textbf{Meaning}  & \textbf{Navigation}\\
    \midrule %%%%%%%%%%%%%%%%%%
    
    (Non-) IID &  (Non-) Independent and Identically Distributed & Sec.~1\\
        
    FedD3 &  Federated Learning from Decentralized Distilled Datasets (Our framework) & Sec.~1\\
    
    ACC &  Prediction Accuracy & Sec.~3\\
    
    \myECEAbbr &  \myECEFull ($\gamma$-\myECEAbbr indicates \myECEAbbr at specific $\gamma$) & Sec.~3\\
    
    DD &  Dataset Distillation  & Sec.~3\\
    
    Img/Cls & Contributed number of distilled images per class from one client  & Sec.~4\\
    
%    KIP &  Kernel Inducing Points & Sec.~\ref{sec:intro}\\
    
    OSFL & One-Shot Federated Learning  & Sec.~4\\
     
    MSFL & Multi-Shot Federated Learning  & Sec.~4\\
    
%    D2D &  Device to Device & Sec.5\\
    
%    D2N &  Device to Networks & Sec.5\\

    %
    \bottomrule %%%%%%%%%%%%%%%%%%
\end{tabular}
\end{threeparttable}
\end{table*}
