# Supplementary material for: Federated Learning via Decentralized Dataset Distillation in Resource-Constrained Edge Environments
Source: arXiv:2208.11311 source file (2023-05-19)
Supplement: Supplementary file 2 [file B_futher_datasets.tex]

\section{Datasets}
\label{subsec:B}

\setcounter{table}{0}

We visualize the distilled images from Fashion-MNIST~\citep{xiao2017/online} in different distillation steps in Fig.~\ref{fig:dd_FashionMnist}.
In Fig.~\ref{fig:further_datasets_vis}, we further visualize the distilled images from decentralized distilled Fashion-MNIST and SVHN, where pathological Non-IID~\citep{huang2021personalized} datasets are distributed in 10 clients. We use five datasets totally for the experiments:
\begin{itemize}
    \item CIFAR-10~\citep{cifar10}: 50000 data points in the training set and 10000 data points in the test set. Each data point is a 32x32 RGB image, associated with a label from 10 classes
    \item Fashion-MNIST~\citep{xiao2017/online}: 60000 data points in the training set and 10000 data points in the test set. Each data point is a 28x28 gray-scale image, associated with a label from 10 classes
    \item MNIST~\citep{mnist-2010}: 60000 data points in the training set and 10000 data points in the test set. Each data point is a 28x28 gray-scale digit image, associated with a label from 10 classes
    \item SVHN~\citep{netzer2011reading}: 73257 data points in the training set and 26032 data points in the test set. Each data point is a 32x32 RGB digit image, associated with a label from 10 classes
    \item CIFAR-100~\citep{netzer2011reading}: 50000 data points in the training set and 10000 data points in the test set. Each data point is a 32x32 RGB image, associated with a label from 100 classes.
\end{itemize}

\setcounter{figure}{0}

\begin{figure*}[h!]
\centering
\includegraphics[trim=0 0 0 0,clip,width=1\linewidth]{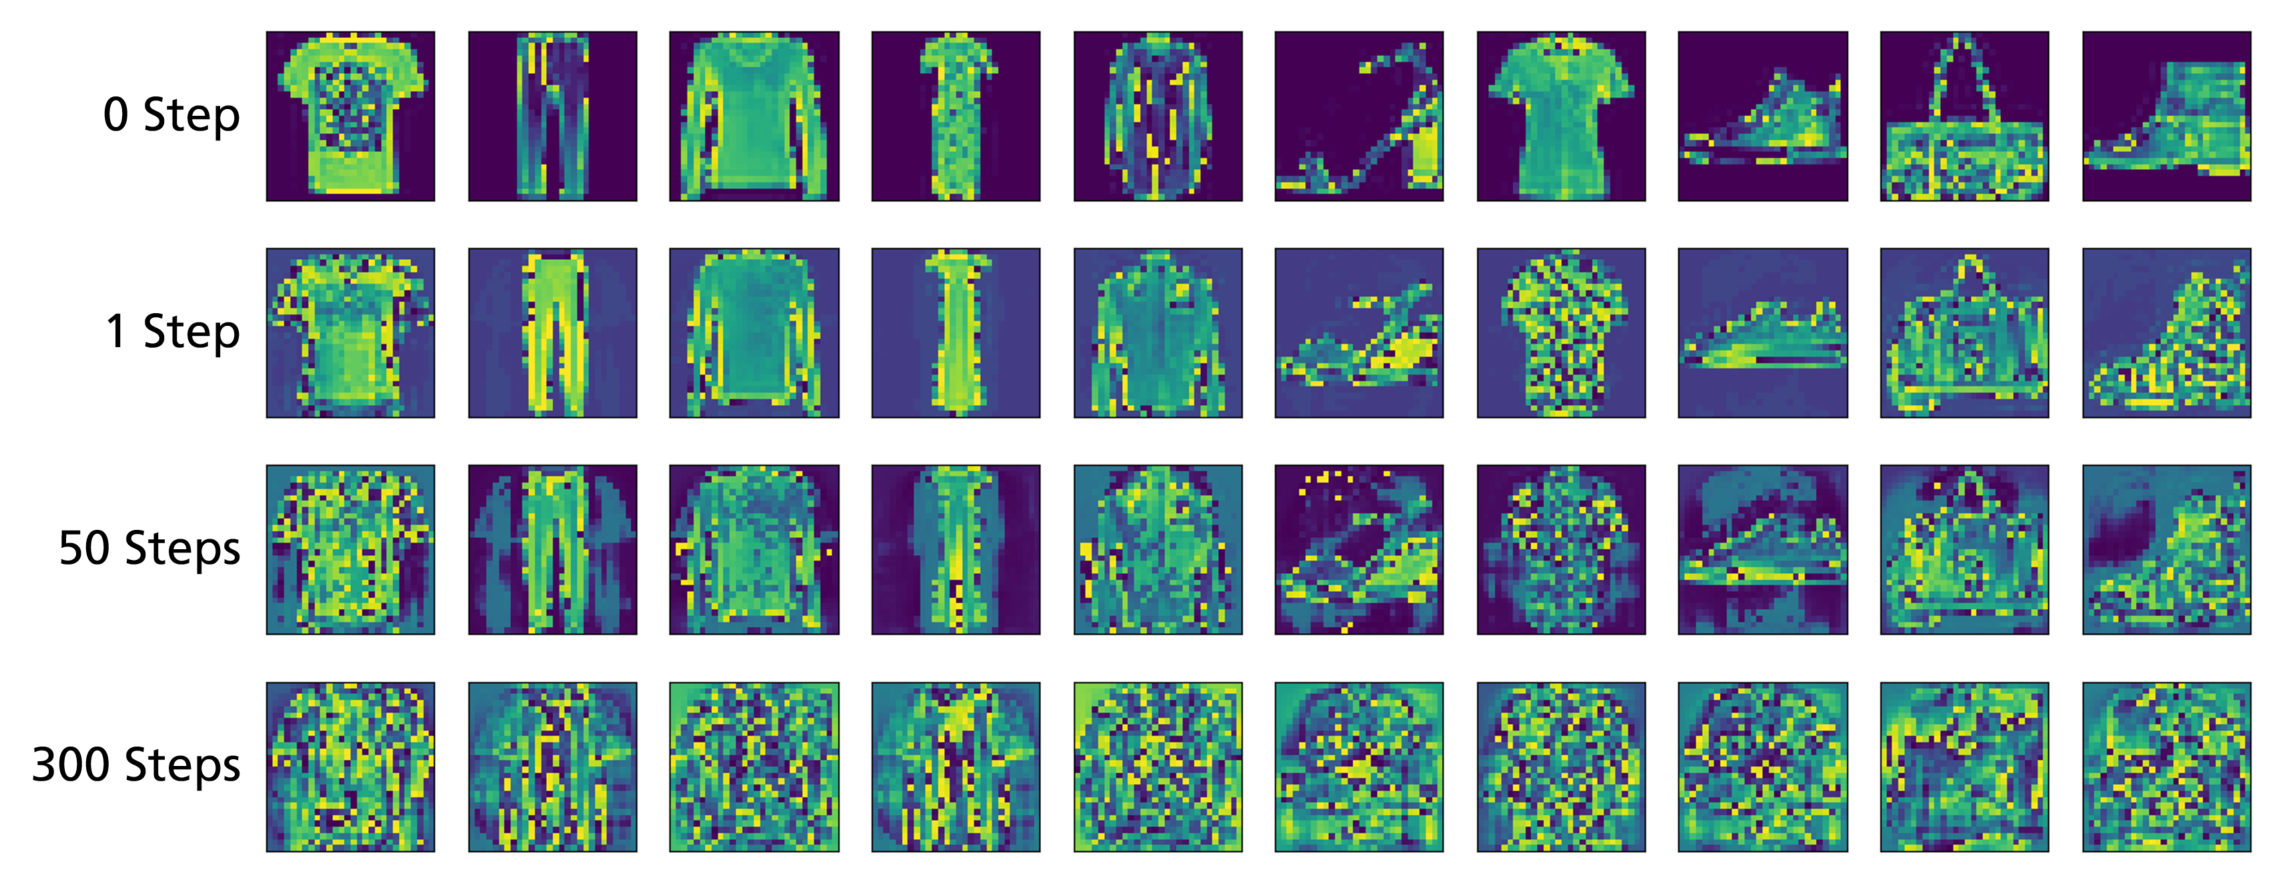}
\caption{Visualization of dataset distillation on IID Fashion-MNIST datasets for 10 classes with increasing distillation steps}
\label{fig:dd_FashionMnist}
\end{figure*}

\begin{figure*}[h!]
\centering
\includegraphics[trim=0 0 0 0,clip,width=1\linewidth]{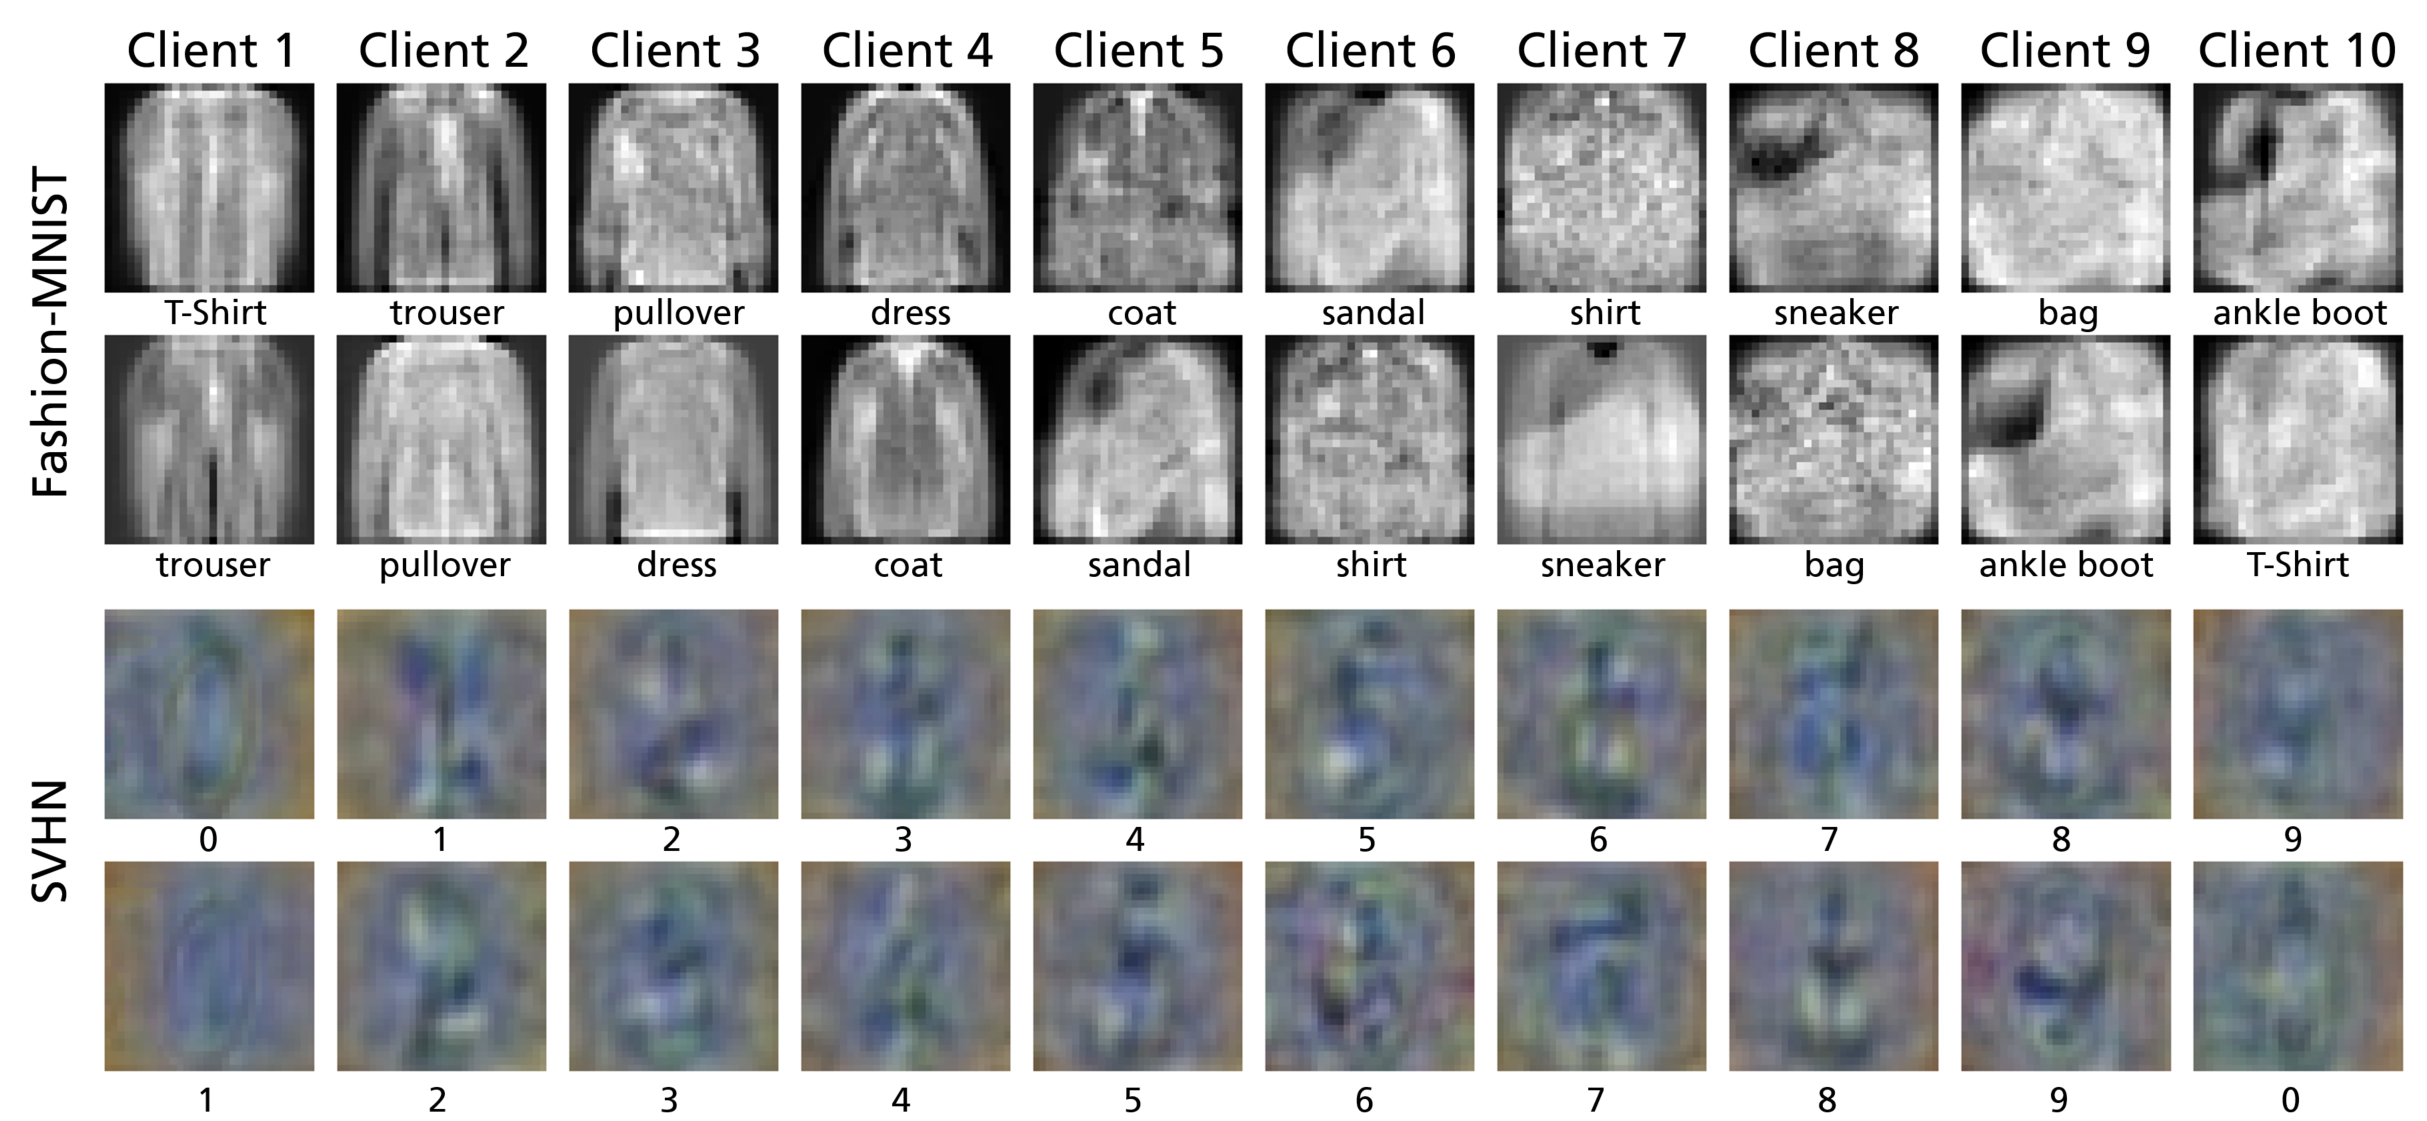}
\caption{Decentralized distilled datasets from 10 clients. The Fashion-MNIST and SVHN datasets are respectively distributed in 10 clients. The local dataset in each client consists of only two classes.}
\label{fig:further_datasets_vis}
\end{figure*}
