# Supplementary material for: Federated Learning via Decentralized Dataset Distillation in Resource-Constrained Edge Environments
Source: arXiv:2208.11311 source file (2023-05-19)
Supplement: Supplementary file 3 [file C_hyperparameters.tex]

\section{Details on Experiments}
\label{subsec:C}

In this section, we report details on datasets, federated system parameters, and hyperparameters in our framework as well as in baselines in our experiments in Sec.~4.3, which run on a computer cluster with 4$\times$~NVIDIA-A100-PCIE-40GB GPUs and 4$\times$~32-Core-AMD-EPYC-7513 CPUs. The environment is a Linux system with Pytorch 1.8.1 and Cuda 11.1.

We divide the datasets (MNIST and CIFAR-10) into 500 clients for model training in federated fashion. 
Considering data heterogeneity across clients, we demonstrate \myFedDD and other baselines on both IID and pathological non-IID~\citep{huang2021personalized} datasets. 
The number of the data points for each class in each client is almost the same, i.e. the data load for 500 clients is nearly balanced. 
For a fair comparison, we do not use any data augmentation methods in \myFedDD and other baselines.
We do not consider any compression methods to enhance the \myECEFull (GCE) equally for \myFedDD and baselines, as it is not the focus of this paper.
In fact, as mentioned in the paper, the standard federated learning (except on-shot federated learning) methods still require communication cost for downloading the global models.
Also, as the type of parameters in images can be uint8 and in models can be float32 or float16 (half precision), the messages for distilled datasets can be compressed smaller.

We compare \myFedDD with eight baselines, four federated learning methods in both one-shot and multi-shot federated fashions. The four methods and the associated parameters are followed: 
(\emph{i}) FedAvg~\citep{pmlr-v54-mcmahan17a}; (\emph{ii}) FedProx~\citep{li2020federated} ($\mu=0.1$); (\emph{iii}) FedNova~\citep{wang2020tackling}; (\emph{iv}) SCAFFOLD~\citep{SCAFFOLD}.

For MSFL, each client trains models on local dataset with fixing 10 epochs between every two communication rounds. 
We use stochastic gradient descent (SGD) with fixing learning rate from $\{0.001, 0.025\}$, momentum 0.9, batch size 50 and number of local epochs from $\{10, 50\}$. 
Note that we use the same learning rate in \myFedDD and baselines for a fair comparison.
we let each test run 10 times with 10 different seeds and use the mean value as the evaluation results.
Considering the communication cost explodes with the increasing communication rounds, only the first 18 and 6 communication rounds for the training on MNIST and CIFAR-10 are considered for the evaluation, respectively, otherwise \myECEAbbr reduces rapidly, due to the increasing of the total communication volume.

For OSFL, the number of local epochs before the one-shot communication matters~\citep{pmlr-v54-mcmahan17a, li2022federated}. The federated learning with more local epochs can train the model more fully in clients, however can lead to overfitting on local datasets. Thus, we set the number of local epochs from $\{1, 10, 50, 100, 150\}$ on MNIST and from $\{1, 5, 10, 20, 50\}$ on CIFAR-10 for all methods.
Specifically for Non-IID MNIST, we have observed the pure one-shot can not achieve good results, as shown in Fig.~2.
%\ref{fig:acc-msg}. 
%
Thus, we run one pre-aggregation for all clients before the OSFL for a much better evaluation results in baselines. 
Each method runs with each of those values 5 times with different seeds.
Finally, only the best 5 results out of 25 tests are considered for the evaluation.

For \myFedDD, we integrate both coreset- and KIP-based instances. We let each client distill only 1 synthetic image per class and upload them to server, i.e. each client contributes 2 distilled images on Non-IID dataset and 10 distilled images on IID dataset.
That also explains why \myFedDD may achieve a better test accuracy but with lower \myECEAbbr on IID dataset than on Non-IID dataset.
Specifically, we use Gaussian mixture model to perform the \myFedDD with coreset-based instance.
For KIP-based instance, we use a 4-layer and 1024-width fully connected model distill the dataset with distillation learning rate 0.004 and batch size 10\% of local dataset size. 
We set a maximum number of epochs on 3000 and a threshold of distillation accuracy on 0.999.
If the threshold is exceeded, the distillation loop breaks out immediately and the client is ready to upload the synthetic images.

Beside the comparison results on MNIST and CIFAR-10 in Tab.3, we further conduct the experiments for training a ResNet-18~\citep{he2016deep} on Fashion-MNIST and SVHN, and training a CNN on CIFAR-100 using MSFL, OSFL and \myFedDD in Tab.4.
Note that for MSFL, We select the best result in the first 3, 9 and 15 communication rounds for the training on Fashion-MNIST, SVHN and CIFAR-100, respectively.
The best results among their corresponding instances are shown in Tab.~3. 
Note that the Img/Cls for the tests on SVHN is 10, other hyperparameters are the same as in Tab.~2.

As we expected, on IID datasets, \myFedDD can achieve comparable test prediction accuracy with much better \myECEAbbr. 
On Non-IID datasets, \myFedDD outperforms both MSFL and OSFL in terms of accuracy and communication efficiency. 
The two biggest advantages of \myFedDD, i.e. communication efficiency and robustness to data heterogeneity, are experimentally validated, which is consistent with the conclusions in Tab.~2.
