# Supplementary material for: Federated Learning via Decentralized Dataset Distillation in Resource-Constrained Edge Environments
Source: arXiv:2208.11311 source file (2023-05-19)
Supplement: Supplementary file 4 [file F_hybrid_fl.tex]

\section{Multi-shot Communication}
\label{subsec:F}

\setcounter{figure}{0}

\begin{figure*}[ht!]
\includegraphics[trim=0 0 0 0,clip,width=1\linewidth]{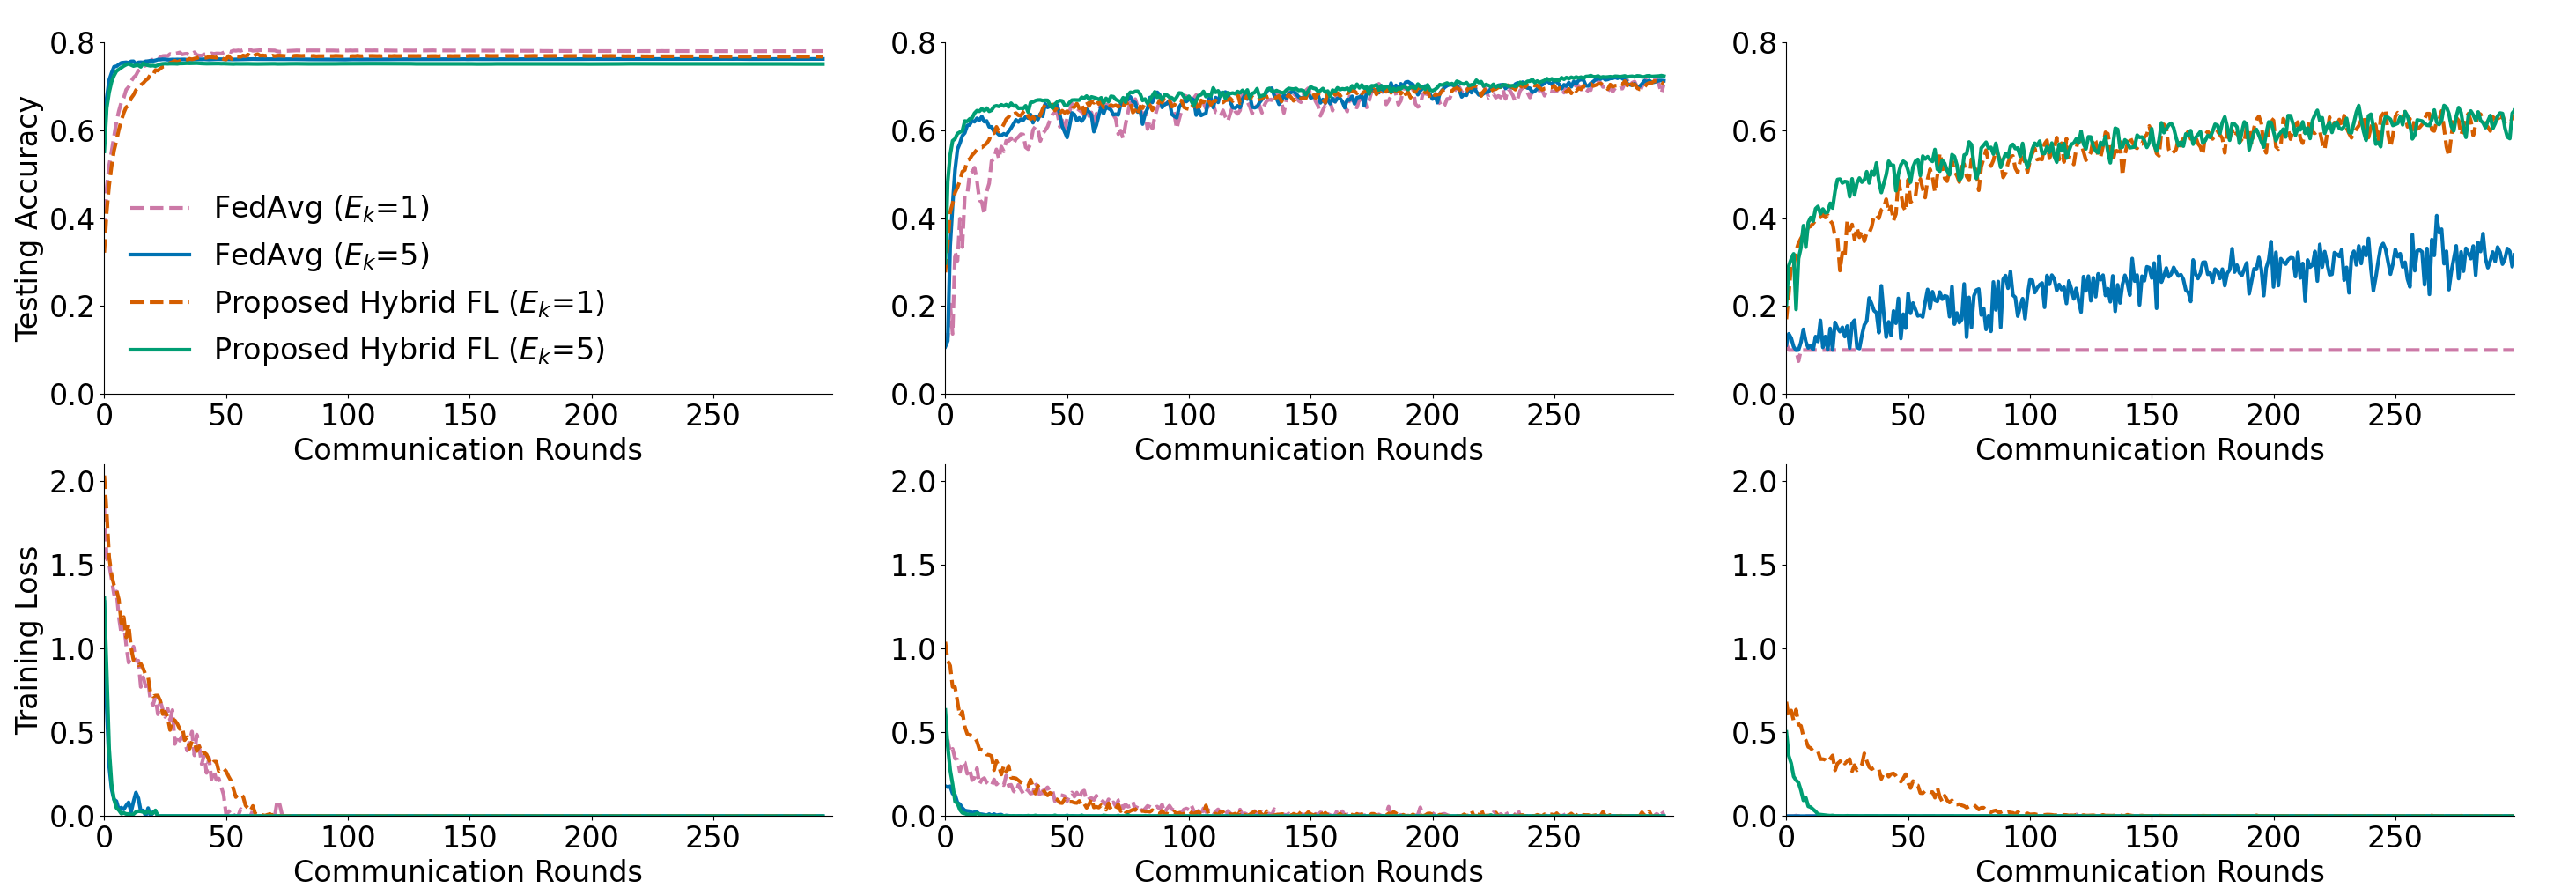}
\caption{The proposed \emph{hybrid federated learning} approach (multi-shot version of \myFedDD) outperforms the standard federated learning on Non-IID decentralized datasets. We consider two local training epoch $E_k$ from $\{1, 5\}$ with batch size $|\mathcal{B}_k|=50$ for each dataset. The Learning rate at $C_k \in \{10, 2\}$ is $0.025$, and at $C_k=1$ is $0.001$.}
\label{fig:hybrid_fl}
\end{figure*}
Due to the robustness on data heterogeneity, we further explore the potential benefits of distilled datasets in federated learning. 
We believe that sharing such synthetic data might bridge the information silos. 
For that, we extend \myFedDD to multiple shots and consider a hybrid federated learning method by adding a spoon of distilled datasets from other clients via D2N (Device to Networks) or D2D (Device to Device) networks.

In particular, in the first communication round, the client $p$ and receive the global model parameters as well as the distilled datasets in other clients $\mathcal{\tilde D}_p^* = \{\mathcal{\tilde D}_k|k \in \mathbb{N}_+, 1 \leq k \leq m, k \neq p \}$ from the server. Thus, for the client $p$, it trains the model on its local dataset $\mathcal{D}_p$ combing with $\mathcal{\tilde D}_p^*$.

%We consider \emph{Hybrid Federated Learning} as one federated learning approach, which extends our \myFedDD to multiple communication rounds. As discussed in \emph{A Spoon of Distilled Datasets into Multi-rounds}, we let the decentralized distilled datasets be aggregated at the server before standard federated learning. In the first communication round, the client $p$ and receive the global model parameters as well as the distilled datasets in other clients $\mathcal{\tilde D}_p^* = \{\mathcal{\tilde D}_k|k \in \mathbb{N}_+, 1 \leq k \leq m, k \neq p \}$ from the server. Thus, for the client $p$, it trains the model on its local dataset $\mathcal{D}_p$ combing with $\mathcal{\tilde D}_p^*$. 

We run \emph{hybrid federated learning} to enhance the baseline \emph{FedAvg}~\citep{pmlr-v54-mcmahan17a} and train an AlexNet model on CIFAR-10 distributed in 10 clients with $C_k$ from $\{10, 2, 1\}$. As the evaluation results shown in Fig.~\ref{fig:hybrid_fl}, though, the \emph{hybrid federated learning} can tiny reduce the convergence speed and test accuracy on IID dataset, the \emph{hybrid federated learning} on Non-IID dataset can notably increase the robustness to data heterogeneity. We also notice that even when the \emph{FedAvg} is failed ($E_k=1$ at $C_k=1$), the \emph{hybrid federated learning} can still be convergence in the training.

We believe the distilled datasets from other clients provide each client an insight of global dataset information. Such a multi-shot version of \myFedDD also reveal that dataset distillation technique can provide an effective strategy for improving federated learning performance on Non-IID datasets.
