# Supplementary material for: Federated Learning via Decentralized Dataset Distillation in Resource-Constrained Edge Environments
Source: arXiv:2208.11311 source file (2023-05-19)
Supplement: Supplementary file 5 [file D_further_comparsion.tex]

\section{Comparison on Further Datasets}
\label{subsec:D}

Beside the comparison results on MNIST and CIFAR-10 in Tab.~\ref{table:comparison}, we further conduct the experiments for training a ResNet-18~\citep{he2016deep} using MSFL, OSFL and \myFedDD on Fashion-MNIST and SVHN. 
Note that for MSFL, We select the best result in the first 3 and 9 communication rounds for the training on Fashion-MNIST and SVHN, respectively.
The best results among their corresponding instances are shown in Tab.~\ref{table:benchmark_further}. 
Note that the Img/Cls for the tests on SVHN is 10, other hyperparameters are the same as in Tab.~\ref{table:comparison}.

As we expected, on IID datasets, \myFedDD can achieve comparable test prediction accuracy with much better \myECEAbbr. 
On Non-IID datasets, \myFedDD outperforms both MSFL and OSFL in terms of accuracy and communication efficiency. 
The two biggest advantages of \myFedDD, i.e. communication efficiency and robustness to data heterogeneity, are experimentally validated, which is consistent with the conclusions in Tab.~\ref{table:comparison}.

\setcounter{table}{0}

\input{appendices/D_1_table_further_comparison}
