# Supplementary material for: Federated Learning via Decentralized Dataset Distillation in Resource-Constrained Edge Environments
Source: arXiv:2208.11311 source file (2023-05-19)
Supplement: Supplementary file 6 [file E_further_models.tex]

\section{Evaluation with Further Models}
\label{subsec:E}

\setcounter{figure}{0}

\begin{wrapfigure}{r}{0.5\textwidth}
\centering
\includegraphics[trim=0 0 0 0,clip,width=1\linewidth]{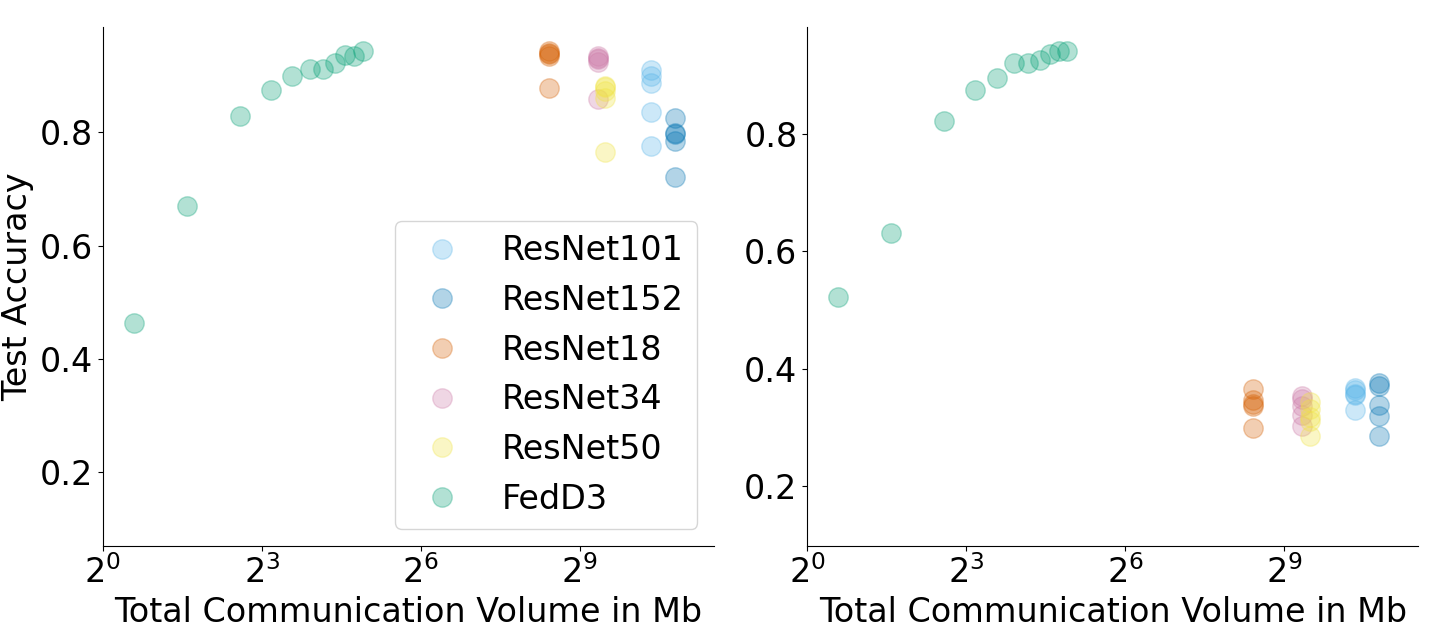}
\caption{Evaluation for OSFL with further model sizes}
\label{fig:ResNet}
\end{wrapfigure}

In this paper, LeNet and AlexNet are mainly used for evaluation, as both of them are compact and can achieve good test accuracy on MNIST and CIFAR-10, respectively. 
Though, the accuracy of one-shot federated learning can still be improved using some large-size models, the required communication volume increases linearly with the size of the model.
In this section, we extend the evaluation in Fig.~2 and compare \myFedDD with one-shot FedAvg for training 5 variants of ResNet~\citep{he2016deep} with $E_k$ from $\{1, 10, 50, 100, 150\}$ on MNIST. 

As in Fig~\ref{fig:ResNet} shown, on IID dataset, the results of one-shot FedAvg are comparable to most of \myFedDD results in terms of test accuracy, however, much larger size of messages for transmitting models is required. 
On Non-IID dataset, \myFedDD outperforms one-shot FedAvg in terms of communication volume notably, as expected.
